# Supplementary material for: Prediction of low energy phase transition in metal doped MoTe$_2$ from first principle calculations
Source: arXiv:1811.07742 source file (2018-11-19)
Supplement: Supplementary file 1 [file main-SM.pdf]

# Supplementary Materials: Prediction of low energy phase transition in metal doped $MoTe_2$ from first principle calculations

Abhinav Kumar[1], Alejandro Strachan[2] and Nicolas Onofrio[1*]

[1] Department of Applied Physics, The Hong Kong Polytechnic University, Hong Kong SAR

[2] School of Materials Engineering and Birck Nanotechnology Center Purdue University, West Lafayette, IN 47906 USA

**Keywords**: *Transition metal dichalcogenides, doping, phase engineering, metal-insulator transition, molybdenum ditelluride*

## Contents

**S1 Charge doping** **2**

S1.1 Constant charge mode . . . . . . . . . . . . . . . . . . . . . . . . . . . . . . 2

S1.2 Constant voltage mode . . . . . . . . . . . . . . . . . . . . . . . . . . . . . . 2

S1.3 Background charge correction . . . . . . . . . . . . . . . . . . . . . . . . . . 2

S1.4 Energy . . . . . . . . . . . . . . . . . . . . . . . . . . . . . . . . . . . . . . 4

S1.5 Validation of SOC approximation . . . . . . . . . . . . . . . . . . . . . . . . 5

**S2 Effect of doping content** **5**

**S3 Kinetics** **6**

**S4 Strain** **7**

*Corresponding author: nicolas.onofrio@polyu.edu.hk

# S1 Charge doping

## S1.1 Constant charge mode

In *constant charge* mode, the monolayer is electrically isolated and charge remains constant during the phase transition. The excess charge can be introduced via external donor/acceptor atoms or molecules [1]. In this case we can directly compare the monolayer energies of H-phase and T'-phase for a given value of excess charge. A simple way to find the critical voltage has been discussed Ref. [2] where the applied voltage is defined as:

$$V(Q) = \frac{Qt}{\epsilon \mathcal{A}} \tag{1}$$

with $t$ the thickness of dielectric material, $\mathcal{A}$ the area and $\epsilon$ the permittivity. For example, the charge density range explored in the paper ($\sigma = \pm 0.08$ e/f.u.) corresponds to voltages between -2.7 and +2.7 V in a capacitor-like setting of 5 nm-thick $HfO_2$ dielectric.

## S1.2 Constant voltage mode

In *constant voltage* mode, the monolayer and the dielectric are sandwiched between two metal plates similar to an electrostatic gating structure [1]. The value of equilibrium excess charge changes during transition but the voltage is fixed. The total energy of the system can be written as:

$$E(Q) = E_{mono}(Q) + \frac{Q^2}{2C} - QW \tag{2}$$

with $E_{mono}$ the energy of the monolayer, $C$ the capacitance and $W$ the work function of the metal plate electrode. The slope of the common tangent of the total energy of each phase function of the excess charge represents the transition voltage, as shown in Figure S1. We note that to access the critical voltage in constant voltage mode one has to correct for the background charge introduced to neutralized the charged supercell (i.e. correct for $E_{mono}$). We summarize the procedure in the following section.

## S1.3 Background charge correction

In VASP, when electrons are added or removed from the system, a compensating background charge is introduced. To get the total energy of the monolayer and therefore, remove the effect of the background

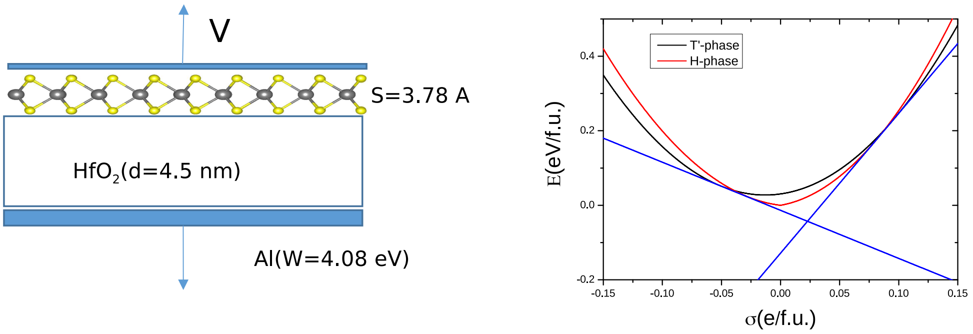


Figure S1: Electrostatic gating structure considered for all constant voltage calculations (left). Total energy (Eq. 2) of H-phase and T'-phase $MoTe_2$ as a function of the charge density (right). The positive and negative critical voltages are extracted from the common tangents.

charge we followed the method prescribed Ref. [1]. The method is well described in the Supplementary Information of the aforementioned reference. In summary, the energy of the monolayer is defined with reference to a plane $z_0$ as:

$$E_{mono}\left(Q, z_0\right) = E_0 + \int_0^Q \Delta V\left(Q', z_0\right) dQ' \tag{3}$$

with $E_0$ the energy of neutral monolayer and $\Delta V\left(Q', z_0\right)$ the corrected potential defined as:

$$\Delta V\left(Q', z_0\right) = \left[V_{tot} - \mu_f\left(Q'\right)\right] - \left[V_{bg}\left(Q', z_0\right) - V_{bg}\left(Q', z_f\left(Q'\right)\right)\right] + \frac{Q'}{2\epsilon\mathcal{A}}\left[z_0 - z_f\left(Q'\right)\right] \tag{4}$$

where $V_{bg}\left(Q', z_0\right) = \frac{Q'}{2\epsilon\mathcal{A}L}\left(z^2 - \frac{L^2}{4}\right)$. All calculations were referenced to $z_0$=17.25 Å. Figure S2 shows the electronic Kohn-Sham potential with and without correction for charged $MoTe_2$ and, Figure S3 shows the corrected and uncorrected H/T' energy differences as a function of the excess charge density corresponding to 6.3 % Mn and Tc doped $MoTe_2$ as well as for pristine $MoTe_2$. The individual H and T' background corrected energy curves as a function of the excess charge are shown Figure S4. The slope of the common tangents yields 1.19, 1.20 and -1.29 V minimum critical voltages to trigger the phase transition in 6.3 % Mn and Tc doped $MoTe_2$ as well as pristine case, respectively. We note that since a background charge is introduced to both H and T' phase supercells, the resulting energy difference is free of background charge, in a first approximation (see Figure S3 and Ref. [2]). Therefore, the energy differences reported Figure 3 in the main paper were not background corrected.

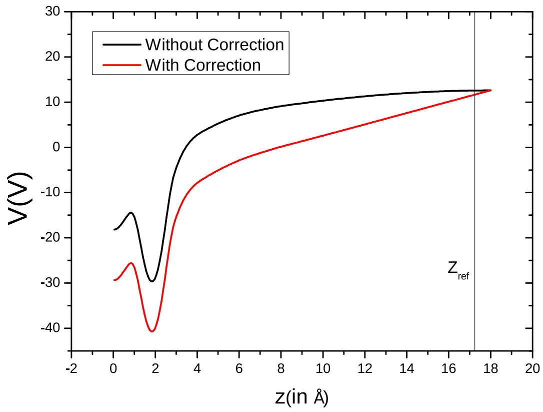


Figure S2: Average electronic Kohn-Sham potential along the vacuum direction $z$ of a ($\sigma = 0.15$ e/f.u.) charged monolayer 2H-$MoTe_2$ with (red) and without (black) background correction.

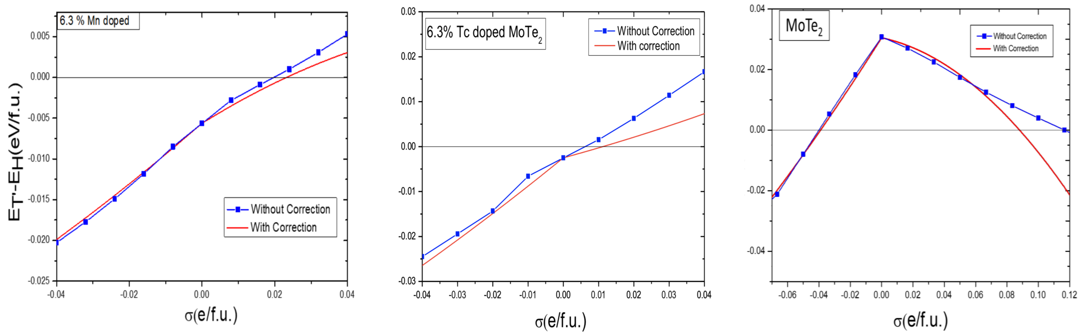


Figure S3: Energy difference between H/T' phases with (red) and without (blue) background correction as a function of excess charge density for 6.3 % Mn and Tc doped $MoTe_2$ as well as pristine $MoTe_2$ (from left to right).

## S1.4 Energy

The method to find the voltage excess charge plot and how to calculate the energy input from the plot is described Ref. [3]. We first find the background corrected total energy of the monolayer for each phase to determine the critical voltage in constant voltage mode. Figure S4 shows the corresponding energies for $MoTe_2$ and 6.3 % Mn doped $MoTe_2$. These energies correspond to a capacitor like structure which includes 4.5 nm thick $HfO_2$ with $\epsilon_r$=25 and, Al-plate with work function of 4.08 eV. The distance between the centre of the monolayer and the dielectric surface is considered as 3.78 Å. The corresponding voltage excess charge diagram are represented Figure S5. The input energy can be extracted by integrating Figure S5 as:

$$E\,(T = 0K) = \int_{GS} V dQ + \int_{mixed} V dQ \tag{5}$$

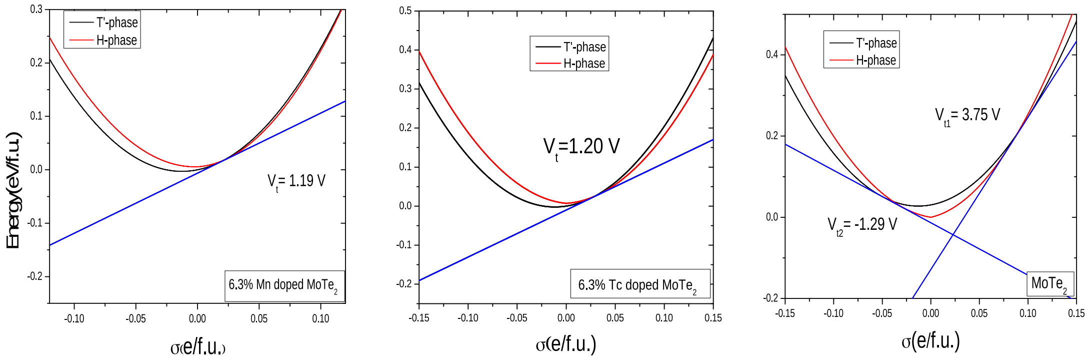


Figure S4: Total energy as a function of excess charge density ($\sigma$) for H-phase and T'-phase of 6.3 % Mn and Tc doped $MoTe_2$ as well as pristine $MoTe_2$ (from left to right).

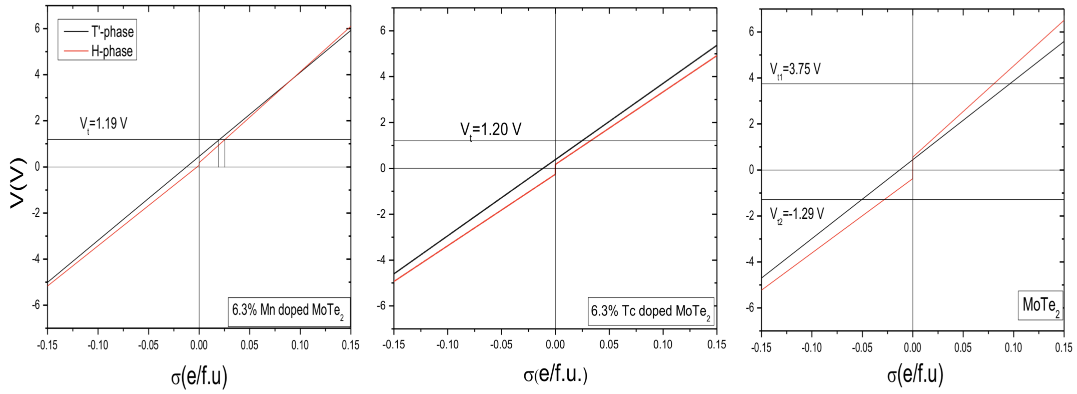


Figure S5: Voltage-excess charge diagram for 6.3 % Mn and Tc doped $MoTe_2$ as well as pristine $MoTe_2$ (from left to right). The energies have been normalized with respect to the bulk volume of ground state structure, considering lattice constant along c-direction as 6.98 Å.

We found energy input of 0.11 (in good agreement with 0.13 in Ref. [3]), 0.062 and 0.048 aJ/nm$^3$ for pristine $MoTe_2$, 6.3 % Tc and Mn doped $MoTe_2$, respectively.

### S1.5 Validation of SOC approximation

Figure S6 shows H/T' energy difference as a function of the excess charge for pristine, 6.3 % Mn and Tc doped $MoTe_2$ monolayers. We can see that the approximated SOC* method is in perfect agreement with calculations fully including SOC.

## S2 Effect of doping content

Figure S7 shows the H/T' energy difference for various dopants at concentrations 4.2, 6.3 and 12.6 %. One can estimate the critical doping concentration (the concentration at which the compound will charge

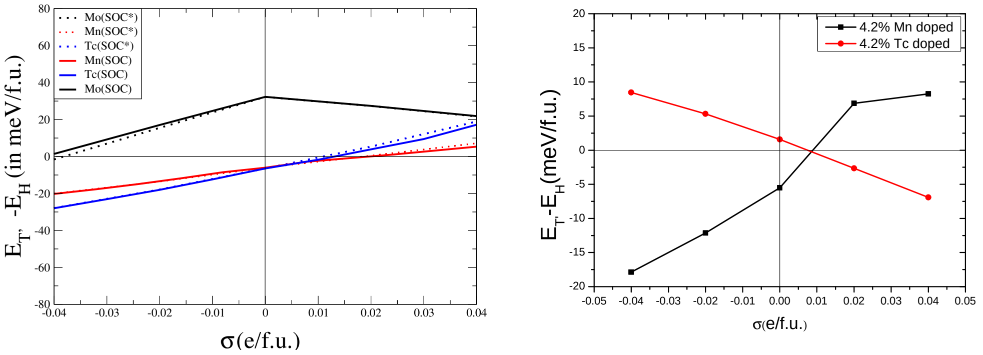


Figure S6: Comparison between SOC* and SOC H/T' energy difference as a function of excess charge for pristine, 6.3 % Mn-doped and 6.3 % Tc-doped $MoTe_2$ (left). SOC calculation of H/T' energy difference as a function of excess charge for 4.2 % Mn and Ti doped $MoTe_2$.

phase) for different dopants as a function of the H/T' energy difference from a simple linear model (see Figures S8 and S9). The critical concentrations for various doped $MoTe_2$ are listed Table S1.

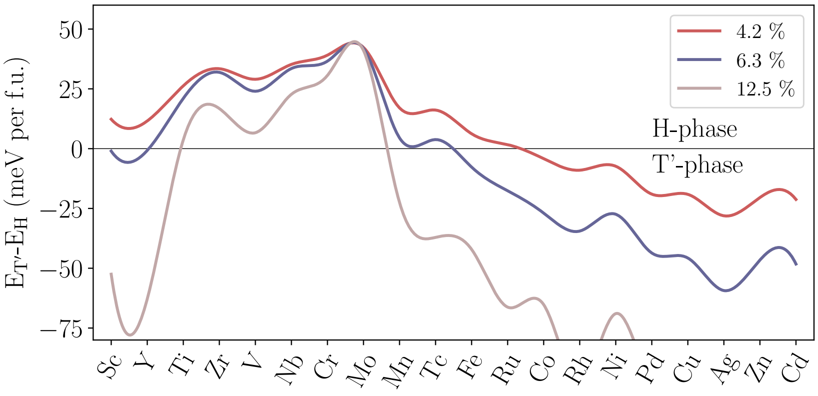


Figure S7: $E_{T'}$-$E_H$ per formula unit at different doping concentrations for various dopant.

# S3 Kinetics

The phase transition timescale ($\tau$) can be calculated using Arrhenius's equation $\frac{1}{\tau} = Ae^{\frac{-E_A}{K_B T}}$ with $A$ a characteristic frequency (taken as 10 Thz), $E_A$ the energy barrier between phases, calculated via NEB calculations (see Figure S10) and, $T$ the temperature at which the transition occurs (here T = 300 K). The activation energy and transition timescale of 6.3 % Sc, Mn and Tc doped $MoTe_2$ as well as pristine $MoTe_2$ are reported Table S2.

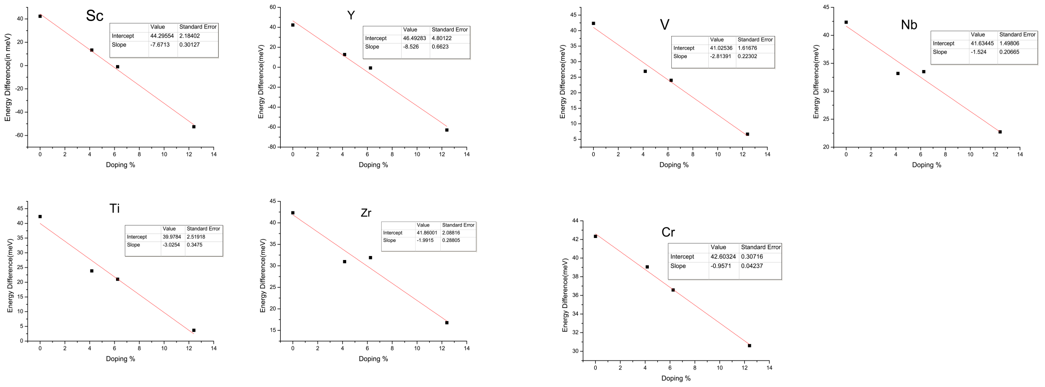


Figure S8: H/T' energy difference per formula unit as a function of dopant concentration for Sc-Cr doped $MoTe_2$.

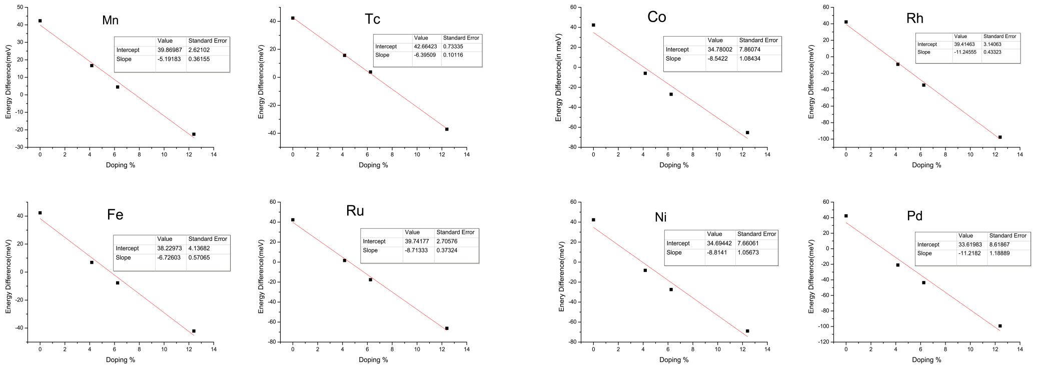


Figure S9: H/T' energy difference per formula unit as a function of dopant concentration for Mn-Pd doped $MoTe_2$.

# S4 Strain

To estimate the critical uniaxial load we used a series of 1D cubic interpolations. To generate Figure 4 of the main paper we computed energies on a 5×5 grid with various lattice constants between -8 % and 8 % with respect to the equilibrium lattice constant. Then we used a cubic polynomial to fit the energies as a function of $a$ for each of the five values of $b$. The minimum values of energies are fitted again as a function of $b$ to get the transition load. Similarly, one can obtain the $a$ transition transition load. Transition loads were normalized with respect to the zero strain lattice parameter of the ground state doped system. This method has been discussed in detail in the Supplementary Information of Ref. [4]. Figures S11 to S18 show the corresponding fits and common tangents used to determine the transition loads for all doped $MoTe_2$ considered in the paper and reported Table 2.

| Dopant | Critical doping concentration % |
|---|---|
| Sc | 5.8 |
| Y | 5.5 |
| Ti | 13.3 |
| Zr | 21.2 |
| V | 14.7 |
| Nb | 27.5 |
| Cr | 45.0 |
| Mo | n/a |
| Mn | 7.7 |
| Tc | 6.7 |
| Fe | 5.7 |
| Ru | 4.6 |
| Co | 4.1 |
| Rh | 3.5 |
| Ni | 3.9 |
| Pd | 3.0 |
| Cu | 2.9 |
| Ag | 2.5 |
| Zn | 2.9 |
| Cd | 2.8 |

Table S1: Critical doping concentration for different dopant. These values have been calculated from linear fitting of energy difference per formula unit for different doping content. We note that these calculation do not include SOC.

| Dopant | Energy Barrier(meV/f.u.) | Time scale($\tau$ in sec) |
|---|---|---|
| Sc | 335 | $4.08 \times 10^{-8}$ |
| Mo | 745 | $3.29 \times 10^{-1}$ |
| Mn | 414 | $8.67 \times 10^{-7}$ |
| Tc | 536 | $1.01 \times 10^{-4}$ |

Table S2: Energy barrier per formula unit and the calculated Transition Time scales have been shown.

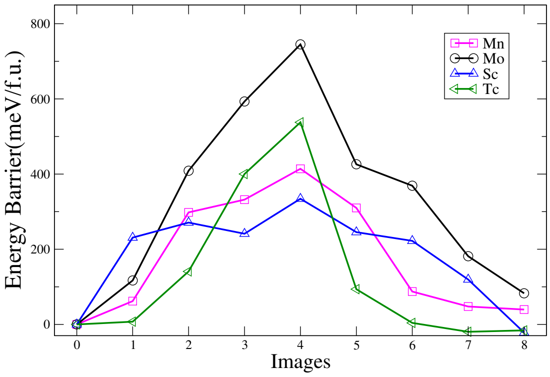


Figure S10: Potential energy surface between H-phase and T'-phase for Mn, Tc, Sc and Pristine $MoTe_2$. The lattice parameters have been fixed to the equilibrium lattice parameters of ground state. All NEB have been performed on a 48 atom unit cell without climbing image method.

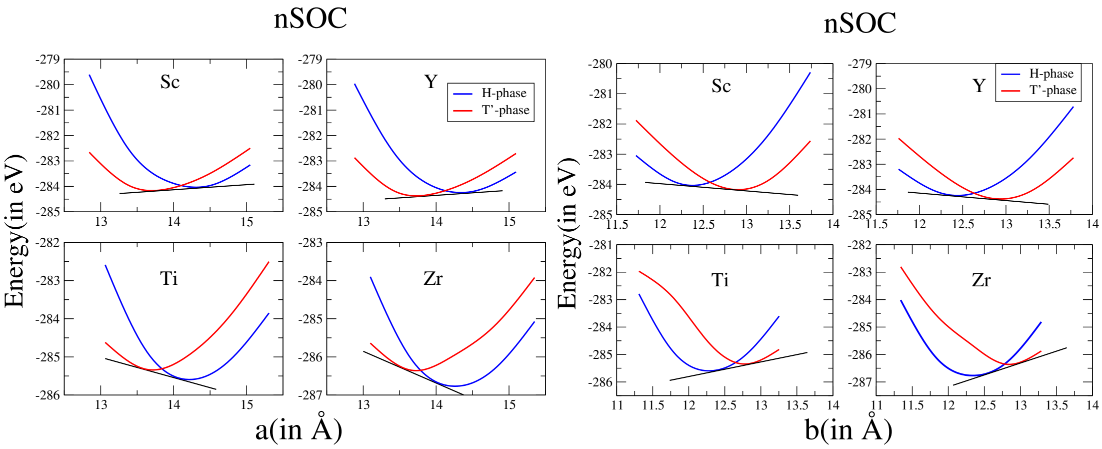


Figure S11: Energy as a function of lattice parameter for 6.3 % Sc-Zr doped $MoTe_2$.

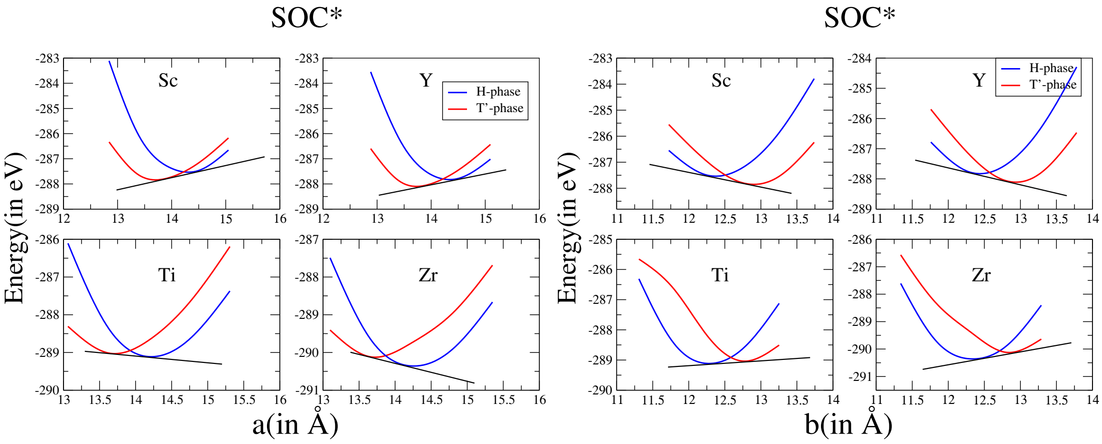


Figure S12: SOC* energy as a function of lattice parameter for 6.3 % Sc-Zr doped $MoTe_2$.

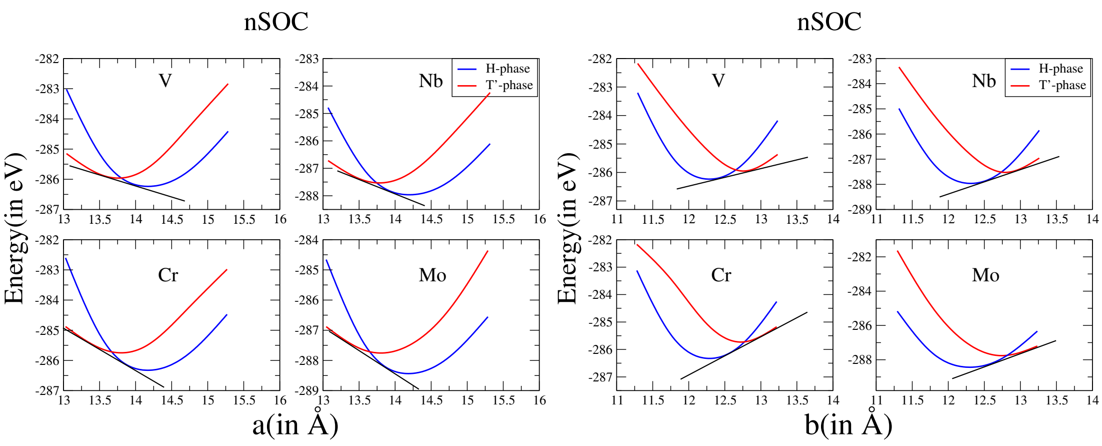


Figure S13: Energy as a function of lattice parameter for 6.3 % V-Mo doped $MoTe_2$.

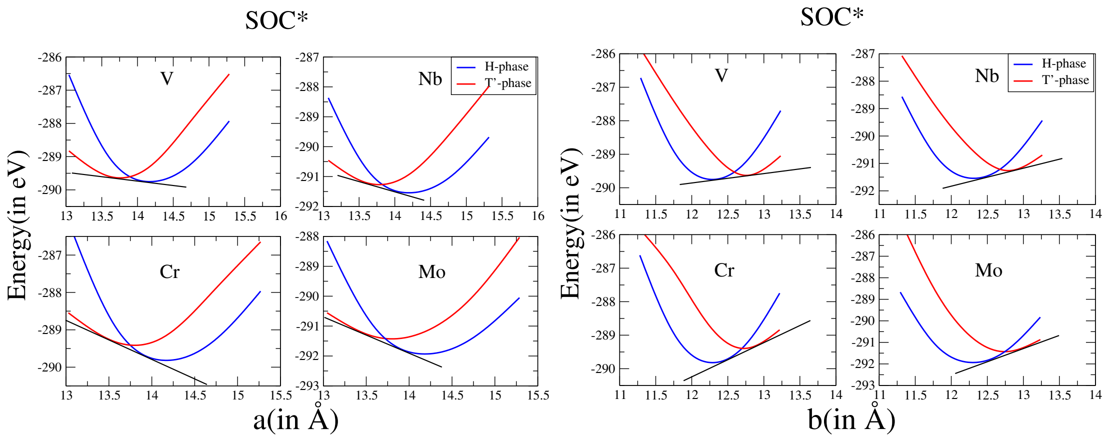


Figure S14: SOC* energy as a function of lattice parameter for 6.3 % V-Mo doped $MoTe_2$.

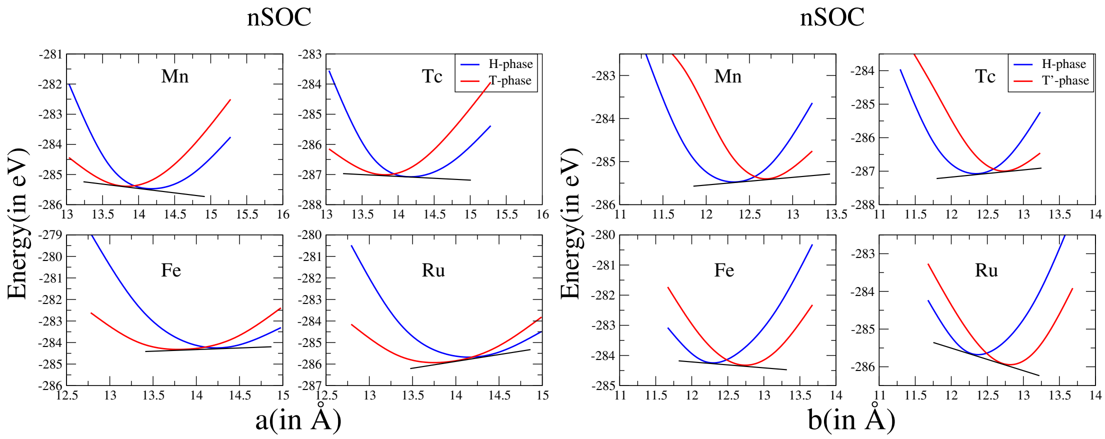


Figure S15: Energy as a function of lattice parameter for 6.3 % Mn-Ru doped $MoTe_2$.

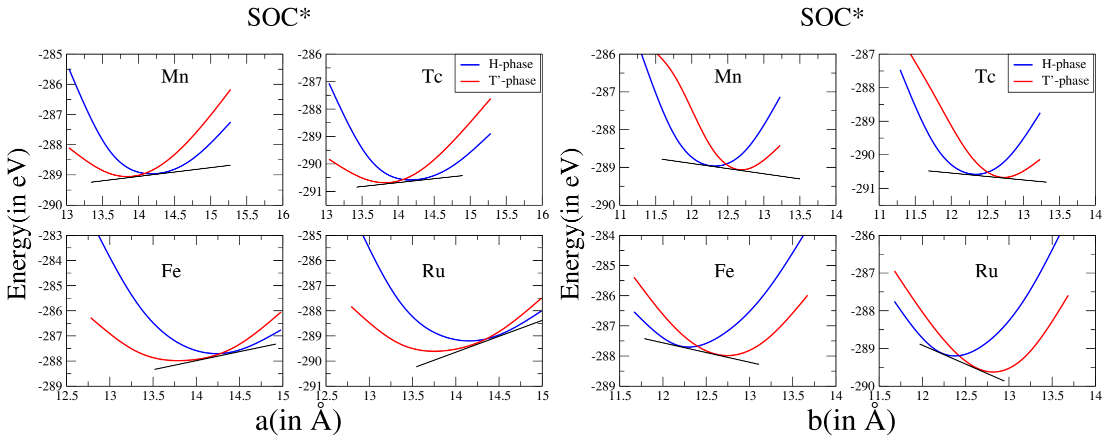


Figure S16: SOC* energy as a function of lattice parameter for 6.3 % Mn-Ru doped $MoTe_2$.

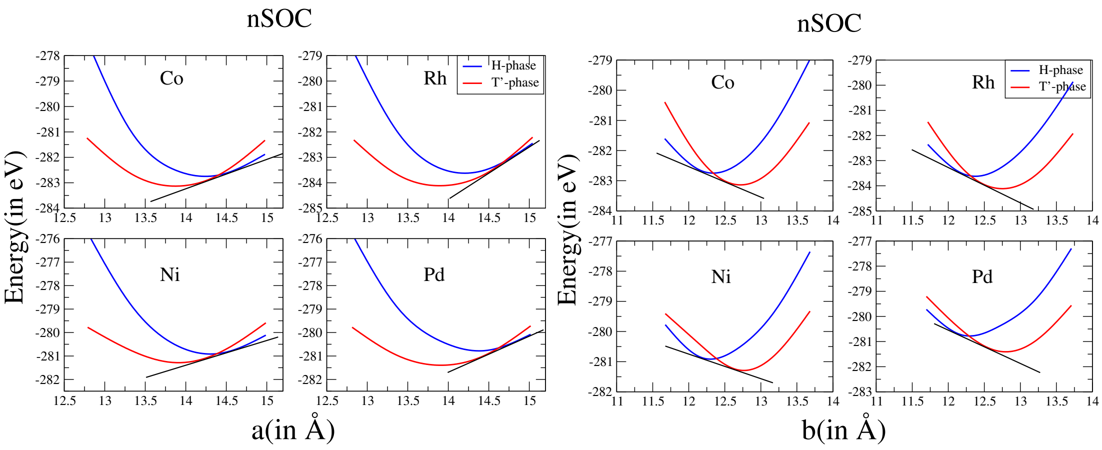


Figure S17: Energy as a function of lattice parameter for 6.3 % Co-Pd doped $MoTe_2$.

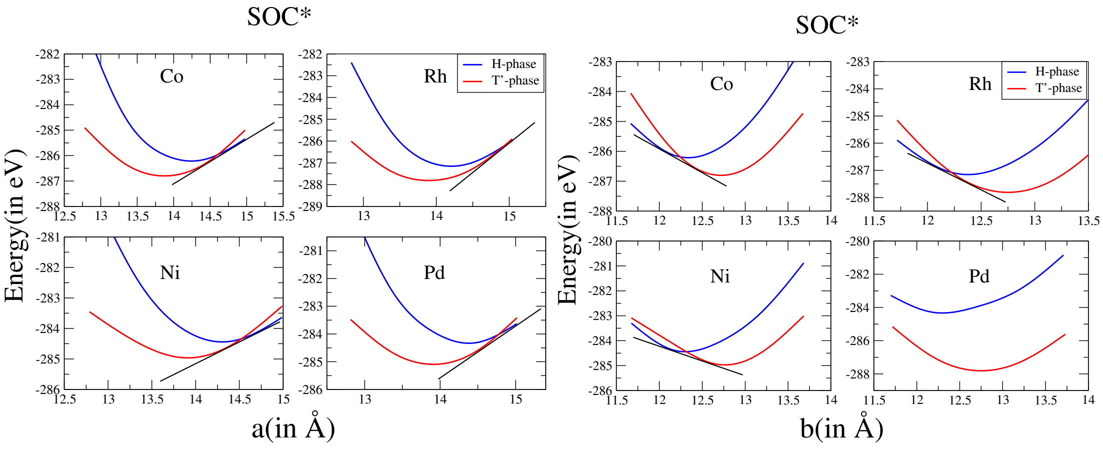


Figure S18: SOC* energy as a function of lattice parameter for 6.3 % Co-Pd doped $MoTe_2$.

# References


[1] Yao Li, Karel-Alexander N Duerloo, Kerry Wauson, and Evan J Reed. Structural semiconductor-to-semimetal phase transition in two-dimensional materials induced by electrostatic gating. *Nature communications*, 7:10671, 2016.

[2] Chenxi Zhang, Santosh KC, Yifan Nie, Chaoping Liang, William G. Vandenberghe, Roberto C. Longo, Yongping Zheng, Fantai Kong, Suklyun Hong, Robert M. Wallace, and Kyeongjae Cho. Charge mediated reversible metal–insulator transition in monolayer mote2 and wxmo1–xte2 alloy. *ACS Nano*, 10(8):7370–7375, 2016.

[3] Daniel A Rehn, Yao Li, Eric Pop, and Evan J Reed. Theoretical potential for low energy consumption phase change memory utilizing electrostatically-induced structural phase transitions in 2d materials. *npj Computational Materials*, 4(1):2, 2018.

[4] Karel-Alexander N Duerloo, Yao Li, and Evan J Reed. Structural phase transitions in two-dimensional mo-and w-dichalcogenide monolayers. *Nature communications*, 5:4214, 2014.
